# Supplementary material for: Mathematics of stable tensegrity structures
Source: arXiv:2101.09616 source file (2023-05-08)
Supplement: Supplementary file 1 [file Appendix.tex]

\section{Linear constraints}
Consider an $m$-dimensional space $\mathcal{V}$. For a bead on cables, $m = 2 \text{ or } 3$ and $\mathcal{V}$ represents the ordinary physical space. However, in tensegrity applications, typically $m = 3N-6$. The vectors $\mathbf{v} \in \mathcal{V}$ represent the small changes representing soft swinging modes. The $c$ linear functions, that approximate the changes in length from its value at $P$, are given to be
\begin{equation}
\mathbf{f}^k : \mathcal{V} \rightarrow \mathbb{R}, \ \forall k=0, \cdots, c-1
\end{equation}
and the condition $\mathbf{f}^k = 0$ is automatically satisfied for the trivial solution $\mathbf{v} = 0$.
